# Supplementary material for: The Random Conditional Distribution for Higher-Order Probabilistic Inference
Source: arXiv:1903.10556 source file (2019-03-25)
Supplement: Supplementary file 1 [file appendix.tex]

\include{operational}
